# Supplementary material for: Rate equations model for multiple magnetic mirrors in various thermodynamic scenarios
Source: arXiv:2105.09614 source file (2022-03-14)
Supplement: Supplementary file 1 [file appendix.tex]

\section{Appendix – numerical details}
